# Supplementary material for: Efficiency of nonparametric superiority tests based on restricted mean survival time versus the log-rank test under proportional hazards
Source: arXiv:2412.06442 source file (2024-12-09)
Supplement: Supplementary file 1 [file rmst_supplementary.pdf]

# Supplementary material for "Efficiency of nonparametric two-sample superiority tests based on restricted mean survival time under proportional hazards"

Dominic Magirr, Craig Wang, Xinlei Deng, Mark Baillie

2024-08-26

## S.1. Plausible scenario leading to $t_H = 4.5$

Consider planning an RCT with one-sided $\alpha = 0.025$, power 0.8, and alternative hypothesis a hazard ratio of 0.67. Applying standard approximations, for 1:1 randomization, the required number of events is 196. Suppose, at the planning phase, a recruitment period of 1.5 years in envisioned, with a further 1.5 years of follow up. Also suppose the event rate on the experimental arm is exponential and the probability of an event at 3 years is predicted to be 0.6 (consistent with the "Moderate" scenario in the simulation study). The R package `rpact` (Wassmer and Pahlke, 2024) can be used to find the required number of patients.

```
plan_A <- rpact::getSampleSizeSurvival(
            alpha = 0.025,
            sided = 1,
            beta = 0.2,
            hazardRatio = 0.67,
            lambda2 = -log(0.6) / 2,
            accrualTime = c(0,1.5),
            followUpTime = 1.5001)

plan_A$maxNumberOfSubjects # => 521.0422
```

```
## [1] 521.0422
```

Now suppose that, in reality, the event rate is only 67% as fast as expected at the design stage. Also suppose that instead of it taking 1.5 years to recruit 521 patients, as planned, it in fact takes 2 years to recruit this number of patients. In this case, the time expected to reach 196 events would approach 4.5 years instead of the 3 years planned.

```
plan_B <- rpact::getSampleSizeSurvival(
            alpha = 0.025,
            sided = 1,
            beta = 0.2,
            hazardRatio = 0.67,
            lambda2 =-log(0.6) / 3,
            accrualTime = c(0, 2),
            accrualIntensity = 521 / 2)

plan_B$studyDuration # =>   4.369084
```

```
## [1] 4.369084
```

## S.2. Flexible parametric survival model details

A Royston & Parmar spline model (Royston, 2001) is used, where the survival distribution on treatment $j = 0, 1$ is modelled as

$$\log(-\log(S(t \mid j))) = s(\log(t), \gamma_j), \tag{1}$$

where $s(\log(t), \gamma_j)$ is a natural cubic spline parameterized by $\gamma_j = (\gamma_{0,j}, \gamma_{1,j}, \gamma_{2,j}, \gamma_3, \gamma_4, \gamma_5)$ with 4 internal knots, and where we allow 3 of the spline parameters to vary with treatment in order to allow for non-proportional hazards.

Using the R package `flexsurv` (Jackson, 2016), this is achieved with the following syntax, with the internal knots are placed at their default locations.

```
## dummy data set
dat <- data.frame(time = rexp(100, 1),
                  event = rep(1,, 100),
                  arm = rep(c("C", "E"), each = 50))


fit <- flexsurv::flexsurvspline(survival::Surv(time, event) ~ arm + gamma1(arm) + gamma2(arm),
                                data = dat, k = 4, scale = "hazard")
```

## S.3. Assessing the proportional hazards assumption in the case studies

## References


Wassmer G, Pahlke F (2024). rpact: Confirmatory Adaptive Clinical Trial Design and Analysis. R package version 4.1.0, https://CRAN.R-project.org/package=rpact.

Royston, P. (2001). Flexible parametric alternatives to the Cox model, and more. The Stata Journal, 1(1), 1-28.

Jackson, C. (2016). flexsurv: a platform for parametric survival modeling in R. Journal of statistical software, 70, 1-33.

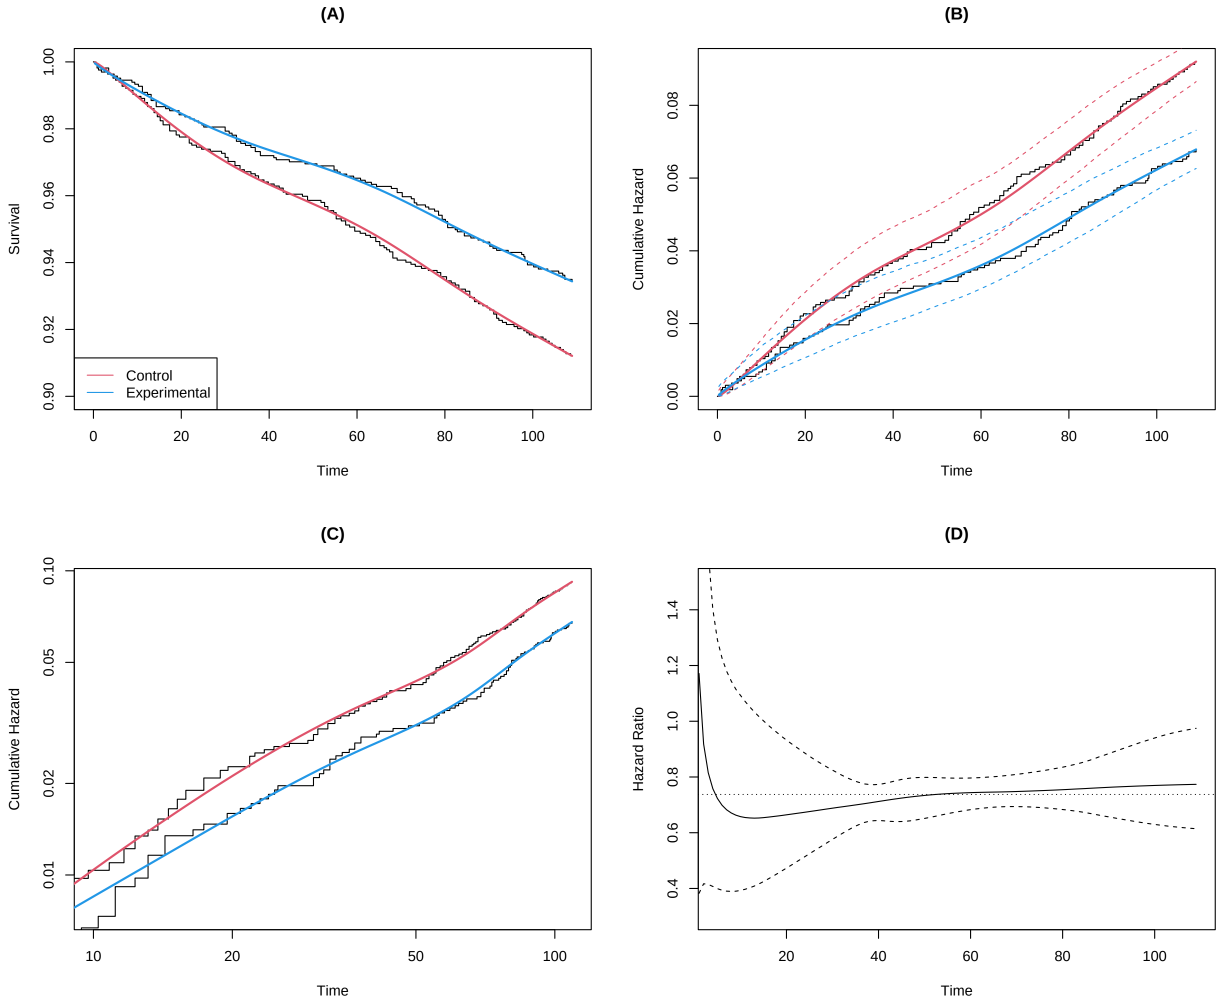


Figure S1: Assessing proportional hazards for the low event-rate, low-censoring example with PH. A: Survival distributions, B: Cumulative hazards, C: Complimentary log-log plot, D: Hazard ratio.

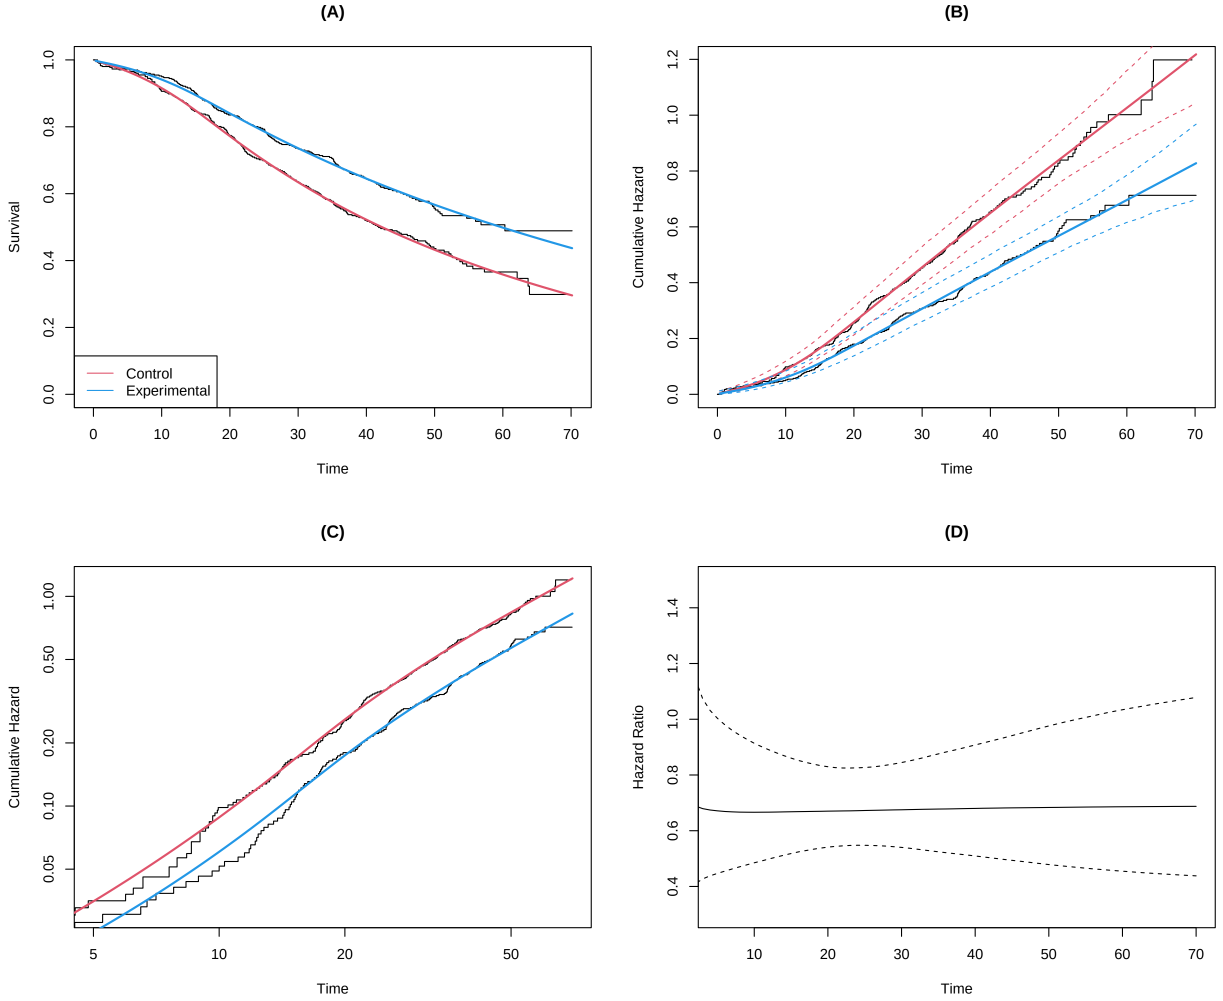


Figure S2: Assessing proportional hazards for the high event-rate, high-censoring example with PH. A: Survival distributions, B: Cumulative hazards, C: Complimentary log-log plot, D: Hazard ratio.

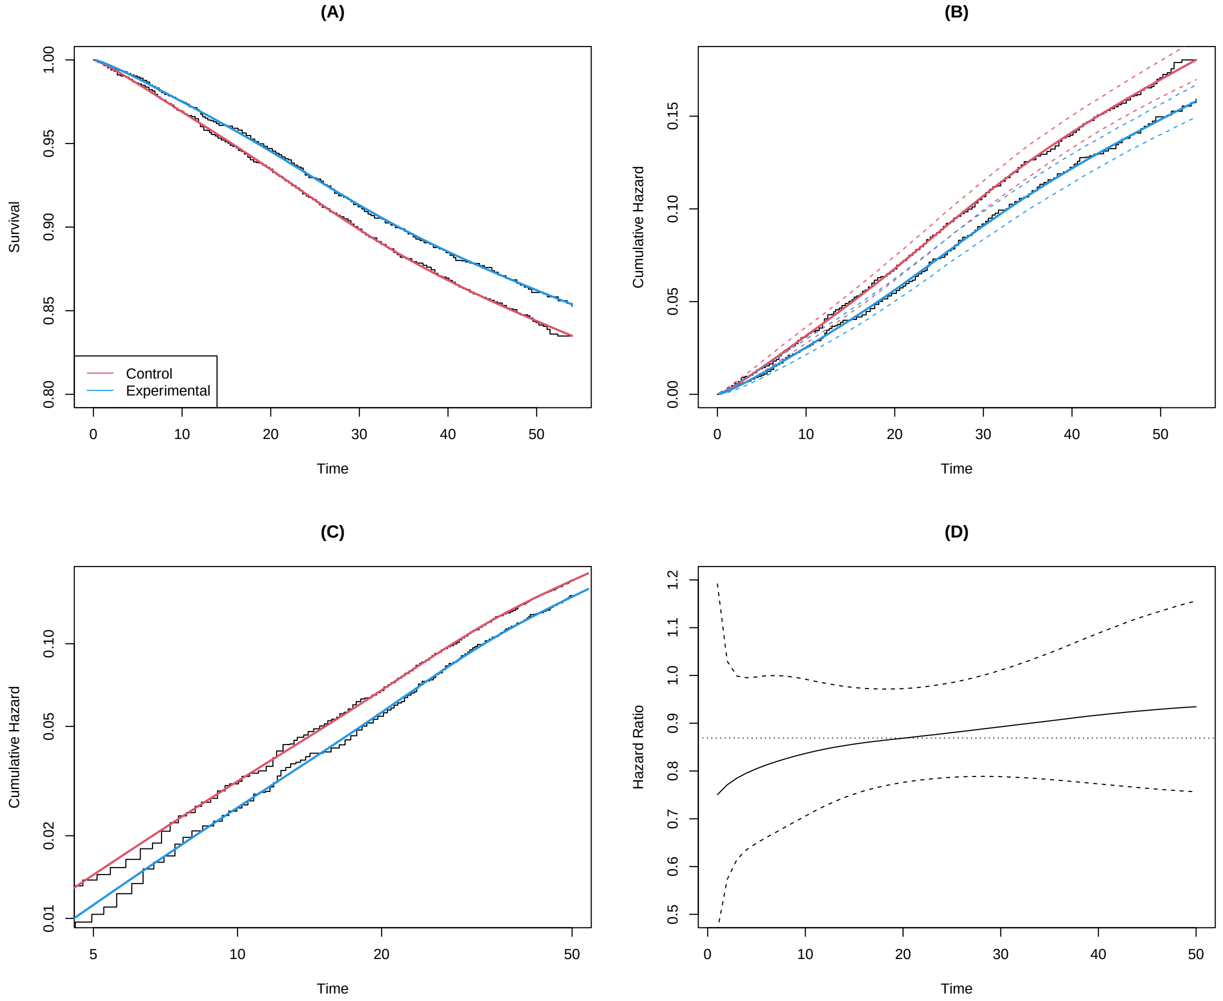


Figure S3: Assessing proportional hazards for the low event-rate, low-censoring example with an early effect. A: Survival distributions, B: Cumulative hazards, C: Complimentary log-log plot, D: Hazard ratio.

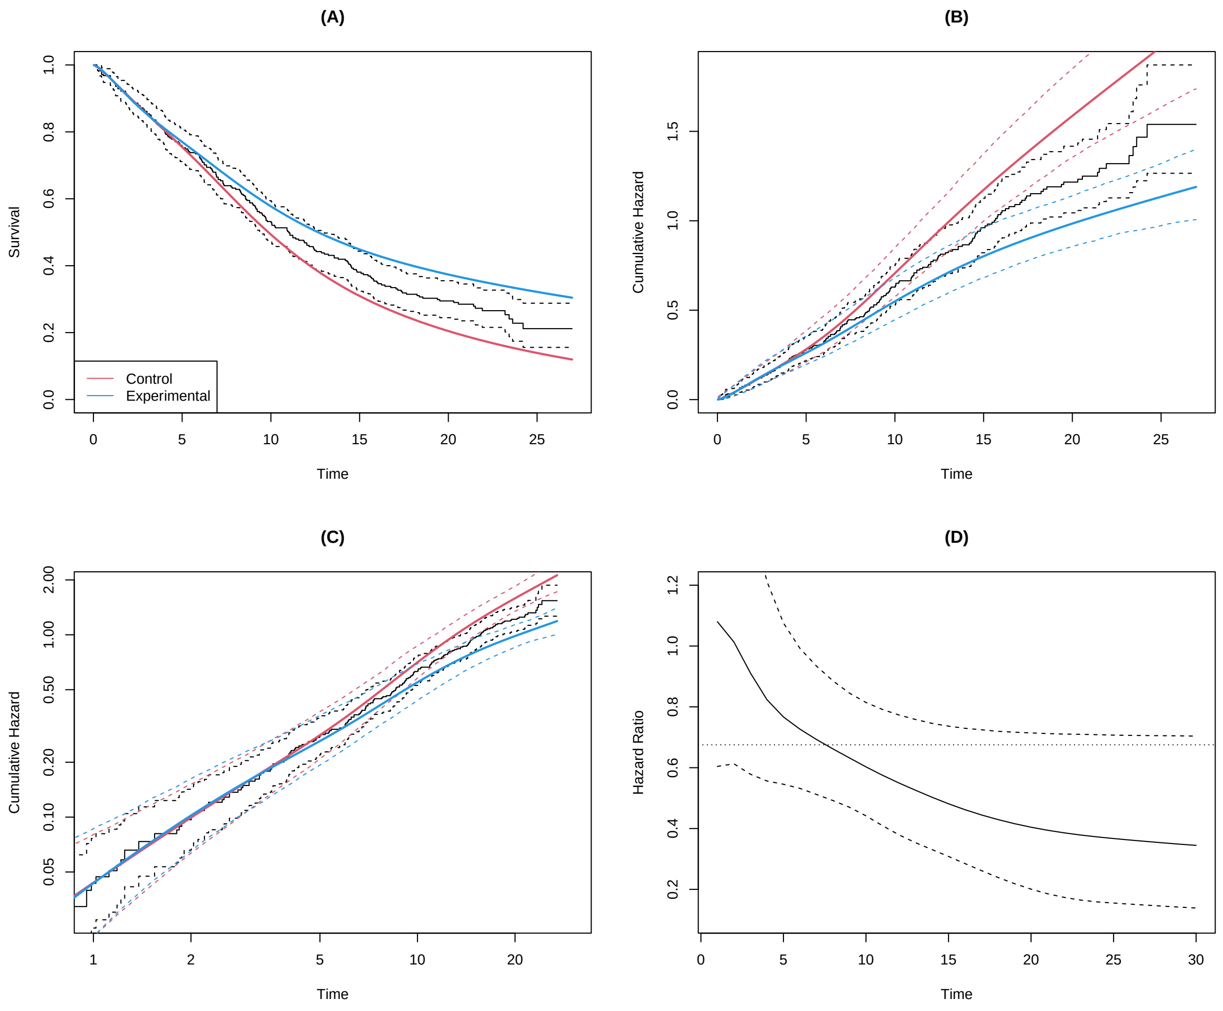


Figure S4: Assessing proportional hazards for the high event-rate, low-censoring example with a delayed effect. A: Survival distributions, B: Cumulative hazards, C: Complimentary log-log plot, D: Hazard ratio.
